# Supplementary material for: Fast Ensembling with Diffusion Schr\"odinger Bridge
Source: arXiv:2404.15814 source file (2024-04-24)
Supplement: Supplementary file 1 [file c10.tex]

\section{Results on CIFAR-10 Dataset}
\label{app:sec:c10}

\begin{table*}[h]
    \newcommand{\metricrule}{\cmidrule(lr){2-3} \cmidrule(lr){4-8}}

    \centering
    \caption{
        Performance on CIFAR-10 dataset.
    }
    \vspace{-2mm}
    \resizebox{\textwidth}{!}{
        \begin{tabular}{lrrllllll}
            \\
            \textbf{CIFAR-10} \\
            \toprule
            Model                 & \dmet{FLOPs} & \dmet{\#Params} & \umet{ACC}          & \dmet{NLL}           & \dmet{BS}           & \dmet{ECE}            & \umet{DEE}           \\
            
            \midrule
            
            ResNet (\gls{de}-1)   & \relv{1.000} & \relv{1.000}    & \tv[n]{91.30}{00.10} & \tv[n]{0.3382}{0.0023} & \tv[n]{0.1409}{0.0011} & \tv[n]{0.0658}{0.0003} & \tv[n]{1.000}{}      \\

            \metricrule

            \quad +2 \gls{bn}\textsubscript{small} (\gls{de}-3)  & \relv{1.125} & \relv{1.097}    & \tv[n]{91.79}{00.05} & \tv[n]{0.2579}{0.0009} & \tv[n]{0.1198}{0.0003} & \tv[n]{0.0599}{0.0037} & \tv[n]{1.899}{}      \\

            \quad +4 \gls{bn}\textsubscript{small} (\gls{de}-5)  & \relv{1.245} & \relv{1.283}    & \tv[n]{91.87}{00.05} & \tv[n]{0.2580}{0.0010} & \tv[n]{0.1195}{0.0004} & \tv[n]{0.0624}{0.0098} & \tv[n]{1.898}{}      \\

            \quad +2 \gls{bn}\textsubscript{medium} (\gls{de}-3)  & \relv{1.411} & \relv{1.319}    & \tv[n]{91.91}{00.04} & \tv[n]{0.2544}{0.0011} & \tv[n]{0.1182}{0.0005} & \tv[b]{0.0591}{0.0096} & \tv[n]{1.938}{}      \\
            
            \quad +1 \gls{dbn} (\gls{de}-3)  & \relv{1.166} & \relv{1.213}    & \tv[b]{92.98}{00.16} & \tv[b]{0.2403}{0.0027} & \tv[b]{0.1084}{0.0013} & \tv[n]{0.0666}{0.0010} & \tv[b]{2.363}{}      \\

            \quad +2 \gls{dbn} (\gls{de}-5) & \relv{1.332} & \relv{1.426}    & \tv[b]{93.23}{00.07} & \tv[b]{0.2247}{0.0005} & \tv[b]{0.1033}{0.0005} & \tv[n]{0.0662}{0.0009} & \tv[b]{3.031}{}      \\

            \gls{ed} (\gls{de}-3)            & \relv{1.000} & \relv{1.000}    & \tv[n]{91.96}{00.42} & \tv[n]{0.3505}{0.0214} & \tv[n]{0.1366}{0.0074} & \tv[n]{0.0674}{0.0037} & \tv[n]{$<$1}{}      \\

            \gls{ed} (\gls{de}-5)            & \relv{1.000} & \relv{1.000}    & \tv[n]{91.86}{00.21} & \tv[n]{0.3577}{0.0083} & \tv[n]{0.1391}{0.0031} & \tv[n]{0.0683}{0.0017} & \tv[n]{$<$1}{}      \\

            \gls{end2} (\gls{de}-3)        & \relv{1.000} & \relv{1.000}    & \tv[n]{91.99}{00.14} & \tv[n]{0.3405}{0.0079} & \tv[n]{0.1358}{0.0026} & \tv[n]{0.0690}{0.0013} & \tv[n]{$<$1}{}      \\
            
            \gls{end2} (\gls{de}-5)        & \relv{1.000} & \relv{1.000}    & \tv[n]{92.11}{00.23} & \tv[n]{0.3313}{0.0057} & \tv[n]{0.1336}{0.0029} & \tv[n]{0.0645}{0.0014} & \tv[n]{1.077}{}      \\

            \gls{de}-2            & \relv{2.000} & \relv{2.000}    & \tv[n]{92.72}{00.13} & \tv[n]{0.2489}{0.0031} & \tv[n]{0.1125}{0.0012} & \tv[b]{0.0484}{0.0010} & \tv[n]{2.000}{}      \\
            
            \gls{de}-3            & \relv{3.000} & \relv{3.000}    & \tv[b]{93.06}{00.14} & \tv[b]{0.2252}{0.0024} & \tv[b]{0.1038}{0.0008} & \tv[b]{0.0469}{0.0012} & \tv[b]{3.000}{}      \\

            \gls{de}-5            & \relv{5.000} & \relv{5.000}    & \tv[b]{93.61}{00.11} & \tv[b]{0.2005}{0.0015} & \tv[b]{0.0951}{0.0004} & \tv[b]{0.0466}{0.0009} & \tv[b]{5.000}{}      \\
            \bottomrule
        \end{tabular}
    }
    \label{tab:c10}
\end{table*}
