# Supplementary material for: Fast Ensembling with Diffusion Schr\"odinger Bridge
Source: arXiv:2404.15814 source file (2024-04-24)
Supplement: Supplementary file 2 [file inference.tex]

\section{The full inference algorithm of~\gls{dbn} method}\label{app:sec:inference}
\blue{
As mentioned in~\cref{sec:main}, we delve into the inference via the~\gls{dbn} method in this section.
We rewrite the~\gls{sde}~\cref{eq:reverse_i2sb} that simulates the path from the source $\bsZ_1$ to the target $\bsZ_0$:
\[
\dee\bsZ_t
&=
\frac{\beta_t}{\sigma_t} \varepsilon_\phi (\bsh_1, \bsZ_t, t) \dee t
+
\sqrt{\beta_t}\dee W_t,
\quad
\bsZ_1\sim p_1 (\bsZ_1|\bsx).
\]
}
